# Supplementary material for: Leaping through tree space: continuous phylogenetic inference for rooted and unrooted trees
Source: arXiv:2306.05739 source file (2024-01-23)
Supplement: Supplementary file 2 [file Appendix.tex]

\section*{Appendix}

\subsection{Background}
\subsubsection*{Binary trees}
A binary tree is a tree where every node has degree 1 or 3, with the possible exception of a single node of degree 2. The nodes of degree 1 are called \textit{leaves}, the nodes of degree 3 are called \textit{internal nodes} and the node of degree 2, if it exists, is called the \textit{root}. A tree with a root is called \textit{rooted}; otherwise, it is called \textit{unrooted}.

In a rooted tree, we define the \textit{generation} of a node to be the path length between that node and the root. We define the \textit{children} of a node $x$ to be any nodes sharing an edge with $x$ with generation one higher than the generation of $x$. We define the \textit{parent} of a node to be any nodes sharing an edge with $x$ with generation one lower than $x$.
\subsubsection*{Phylogenetic inference}
We consider a tree with $n$ taxa with names $N_0,...,N_{n-1}$. Initially, we suppose that the leaf node corresponding to the taxon with name $N_i$ has label $i$. A phylogenetic tree is a representation of the evolutionary history of these taxa. It is a binary tree where each of the leaves correspond to a taxon. Depending on the problem under consideration, it may be either rooted or unrooted.

Introduced in~\parencite{penn2023}, Phylo2Vec provides a bijective mapping between the space of rooted phylogenetic trees with $n$ taxa and integer-valued vectors $\boldsymbol{v}$ satisfying
\begin{equation}
    v_0 = 0 \quad \text{and} \quad v_m \in \{0,1,...,2(m-1)\}\quad \forall m \in \{1,...,n-1\}
\end{equation}
Hence, we are able to refer uniquely to a rooted tree by its vector representation $\boldsymbol{v}$. As discussed in~\parencite{penn2023}, for a given unrooted tree, there are $2n-1$ vectors which, when the root of the corresponding tree is removed, result in this unrooted tree.

In balanced minimum evolution (BME), traditionally applied to unrooted trees (though we justify its use for rooted trees in the following section), we are provided with a matrix $D$ giving the distance between each pair of taxa. For a given tree, we also calculate the matrix $e$, giving the (unweighted) path length between the leaf nodes corresponding to each pair of taxa. The objective value of this tree is then $f(\boldsymbol{v}) = \sum_{ij}D_{ij}2^{-e_{ij}}$, and the aim of our optimisation algorithm is to find the tree which minimises $f$. 
\subsection{BME for rooted trees}\label{sec:bme_rooted}
\subsubsection*{A rooted tree via a distant ancestor}
The application of BME is almost always restricted to unrooted trees~\parencite{Semple2004-my}. However, we present below a justification for its use in rooted tree space also. Suppose that we have a set of $n$ taxa labelled $\{0,1,..., n-1\}$. We introduce a new taxon, labelled $n$, which is considered a very distant root. Under the (almost always biologically reasonable) assumption that the root evolved long before the other taxa, this root will be approximately independent of all the other taxa. That is, we expect
\begin{equation}
    D_{ni} = D^* + O(\epsilon) \quad \forall i \neq n
\end{equation}
for $\epsilon << 1$, where $\epsilon$ includes both the error from the root not being completely independent of the taxa, and also the aleatoric error in the distance between two independent species. If our distance matrix were based on genetic sequence data, we would need the sequence to be sufficiently long to ensure this aleatoric error was small. This result holds regardless of the distances between the other taxa. Hence, note that, for any unrooted tree with internode path lengths $e_{ij}$,
\begin{align}
    \sum_{i,j}D_{ij}2^{-e_{ij}} &= \sum_{j}D_{nj}2^{-e_{nj}} + \sum_{i}D_{in}2^{-e_{in}} + \sum_{i,j < n}D_{ij}2^{-e_{ij}}\\
    &= \sum_{j}(D^* + O(\epsilon))2^{-e_{nj}} + \sum_{i}(D^*+O(\epsilon))2^{-e_{in}} + \sum_{i,j < n}D_{ij}2^{-e_{ij}}
\end{align}
We can make progress with this sum by noting the Kraft Equality, found throughout the literature~\parencite{catanzaro2012} 
\begin{equation}
    \sum_{j}2^{-e_{nj}} = \frac{1}{2}
\end{equation}
This means that
\begin{equation}
    \sum_{i,j}D_{ij}2^{-e_{ij}} = \sum_{i,j < n}D_{ij}2^{-e_{ij}} + \frac{D^*}{2} +  O(\epsilon)
\end{equation}
Moreover, if there exists some small $\delta$ such that
\begin{equation}
    | D_{na} - D^*| \leq\delta \quad \forall a \neq n
\end{equation}
then a similar argument shows
\begin{equation}
    \bigg|\sum_{i,j}D_{ij}2^{-e_{ij}} - \sum_{i,j < n}D_{ij}2^{-e_{ij}} - \frac{D^*}{2}\bigg| \leq \frac{\delta}{2}
\end{equation}
Thus, provided that there is a unique optimal tree $\mathcal{T}$ minimising $\sum_{i,j}D_{ij}2^{-e_{ij}}$, the finiteness of tree space ensures that, for sufficiently small $\delta$, $\mathcal{T}$ is also the unique minimiser of $\sum_{i,j < n}D_{ij}2^{-e_{ij}}$. 

Hence, assuming the existence of a sufficiently distant ancestor (and assuming sufficiently small aleatoric error) the optimal unrooted tree for the $n+1$ taxa can be found by finding the optimal \textit{rooted} tree for $n$ taxa with the objective function $\sum_{i,j < n}D_{ij}2^{-e_{ij}}$ - that is, the standard BME objective applied to rooted trees with $n$ taxa. This means that the BME objective function can be applied to rooted trees, even though the addition of the root means that it is no longer equal to the tree length. Moreover, applying it in this way provides a way, in theory, to find the root of a set of taxa as this root node is, in our $n+1$ taxa tree, joined to the distant ancestor which we know is the true outgroup. However, as discussed in the following sections, this root may be incorrect when different branches on the tree had different evolutionary rates.
\subsubsection*{The rooting problem}
Suppose we have an unrooted tree $\mathcal{T}$ and that we want to find the optimal rooting for this tree – that is, the edge in the tree such that placing the root on this edge minimizes the BME objective.

Choose an edge, $b$ on which to place the root. We define a function $X_b$ such that $X_b(A,B)$ is 1 if $b$ is on the path between nodes $A$ and $B$. Adding a root to edge $b$ changes the objective function by halving the weight assigned to each $D_{AB}$ such that $X_b(A,B) = 1$ as the path length between these nodes will increase by 1. Thus, using $f_r$ to denote the rooted objective and $f_u$ to denote the unrooted objective,
\begin{equation}
    f_r = f_u - \frac{1}{2}\sum_{X_b(A,B) = 1}D_{AB}2^{-e_{AB}}
\end{equation}
where the $e_{AB}$ are the path lengths in the original, unrooted tree and both $A$ and $B$ are allowed to vary in the sum. Hence, for a fixed unrooted tree topology, the optimal rooting will solve
\begin{equation}
\label{eq:rooting}
    \max_b\bigg\{\sum_{X_b(A,B) = 1}D_{AB}2^{-e_{AB}}\bigg\}
\end{equation}
\subsubsection*{Reformulating the rooting problem}
To make progress in interpreting the solution to the rooting problem (\ref{eq:rooting}), we use the common BME assumption that in the optimal unrooted tree $\mathcal{T}$, there exist edge weights such that $D_{AB}$ is the length between nodes $A$ and $B$ in the tree $\mathcal{T}$ (practically, BME arises from a least squares approximation to these lengths). 

\textbf{Claim:} If $D_{Ar}$ is the distance between node $A$ and the root, and $g_A$ is the path length (i.e. the generation of node $A$), then
\begin{equation}
\label{eq:root_reform}
    \sum_{X_b(A,B) = 1}D_{AB}2^{-e_{AB}} = 2\sum_A2^{-g_A}D_{Ar}
\end{equation}
\textbf{Proof:} Again, the $e_{AB}$ terms refer to the path lengths in the original unrooted tree. (\ref{eq:root_reform}) can be proved by induction on the number of leaf nodes, $n$. For $n=2$, the root must be placed on the edge connecting nodes $0$ and $1$ and $e_{01} = 1$. Then
\begin{equation}
     \sum_{X_b(A,B) = 1}D_{AB}2^{-e_{AB}} = \frac{1}{2}(D_{01} + D_{10})  =\bigg(2^{1-1}D_{0r} + 2^{1-1}D_{1r}\bigg)
\end{equation}
as required, noting that $D_{0r} + D_{1r} = D_{01}$. Suppose that our claim holds for $n = k$ and consider a tree with $n = k+1$. Choose a pair of sibling leaf nodes (i.e. leaf nodes joined to the same internal node) $y$ and $z$ such that the root is not on an edge joining one of these nodes to the tree (this must exist as, for $n > 2$, there are at least two pairs of sibling leaf nodes). Suppose that $y$ and $z$ are connected to the internal node $w$. Now, note that the contribution to the objective of node $y$ is
\begin{align}
    2\sum_{B:X_b(y,B) = 1}D_{yB}2^{-e_{yB}} &= 2\sum_{B:X_b(w,B) = 1}(D_{wB} + D_{wy})2^{-e_{yB}}\\
    &= 2\sum_{B:X_b(w,B) = 1}D_{wB}2^{-e_{yB}} + 2D_{wy} \sum_{B:X_b(w,B) = 1}2^{-e_{yB}}\\
    \label{eq:final_sum} &= \sum_{B:X_b(w,B) = 1}D_{wB}2^{-e_{wB}} + 2D_{wy} \sum_{B:X_b(w,B) = 1}2^{-e_{yB}}
\end{align}
where the factor of $2$ comes from the fact that both $(y,B)$ and $(B,y)$ must be considered. The final term in this equation can be simplified. Consider the subtree whose leaves are the root and all nodes such that $X_b(w,B) = 1$. Then, by the Kraft Equality on this subtree
\begin{equation}
    \sum_{B:X_b(w,B) = 1}2^{-g_B} =\frac{1}{2}
\end{equation}
as $g_B$ gives the distance between the root and node $B$. Moreover, as $e_{yB} = g_y + g_B - 1$ (where the $-1$ accounts for the fact that $\mathcal{T}$ is unrooted)
\begin{equation}
    \sum_{B:X_b(w,B) = 1}2^{-e_{yB}} =  2^{1-g_y}\sum_{B:X_b(w,B) = 1}2^{-g_B} = 2^{-g_y}
\end{equation}
Thus, (\ref{eq:final_sum}) becomes
\begin{equation}
   2 \sum_{X_b(y,B) = 1}D_{yB}2^{-e_{yB}} =  \sum_{B:X_b(w,B) = 1}D_{wB}2^{-e_{wB}} + 2D_{wy}2^{-g_y}
\end{equation}
Thus, the change to $\sum_{X_b(A,B) = 1}D_{AB}2^{-e_{AB}} $ caused by adding nodes $y$ and $z$ from the tree is to subtract
\begin{equation}
    2\sum_{X_b(w,B) = 1}D_{wB}2^{-e_{wB}}
\end{equation}
(as node $w$ is no longer a leaf node) and to add the contributions from nodes $y$ and $z$
\begin{equation}
    2\bigg(\sum_{B:X_b(y,B) = 1}D_{yB}2^{-e_{yB}}  +  \sum_{B:X_b(z,B) = 1}D_{zB}2^{-e_{zB}}\bigg)  =  \sum_{X_b(w,B) = 1}D_{wB}2^{-e_{wB}} + 2D_{wy}2^{-g_y} + \sum_{X_b(w,B) = 1}D_{wB}2^{-e_{wB}} + 2D_{wz}2^{-g_z}
\end{equation}
There is no $(y,z)$ term to consider as $X_b(y,z) = 0$. Note that the $\sum_{X_b(w,B) = 1}D_{wB}2^{-e_{wB}}$ terms cancel. Define   $\mathcal{T}'$ to be the tree when node $y$ and $z$ are removed so, as it now has $k$ leaf nodes, the inductive hypothesis can be used to show
\begin{align}
    \sum_{A,B\in \mathcal{T}:X_b(A,B) = 1}D_{AB}2^{-e_{AB}} &=  \sum_{A',B' \in \mathcal{T}':X'_b(A',B') = 1}D_{A'B'}2^{-e'_{A'B'}} + 2D_{wy}2^{-g_y} + 2D_{wz}2^{-g_z}\\
    &= 2\sum_{A' \in \mathcal{T}'}2^{-g'_{A'}}D_{A'r'}+ 2D_{wy}2^{-g_y} + 2D_{wz}2^{-g_z}\\
     &= 2\sum_{A' \in \mathcal{T}'/\{w\}}2^{-g'_{A'}}D_{A'r'}+ 2D_{wr}2^{-g_w}+ 2D_{wy}2^{-g_y} + 2D_{wz}2^{-e_{zr}} 
\end{align}
where dashes are used to denote quantities in $\mathcal{T}'$. Note that 
\begin{equation}
    \sum_{A' \in \mathcal{T}'/\{w\}}2^{-g'_{A'}}D_{A'r'} = \sum_{A \in \mathcal{T}/\{y,z\}}2^{-g_{A}}D_{Ar}
\end{equation}
as only the nodes $w$, $y$ and $z$ are affected by changing from $\mathcal{T}$ to $\mathcal{T}'$. Moreover, note that
\begin{equation}
    2^{-g_w} = 2^{-g_y} + 2^{-g_z}
\end{equation}
as $g_w = g_y-1 = g_z-1$, and, as the distances are additive,
\begin{equation}
    D_{wy} + D_{wr} = D_{yr} \quad \text{and} \quad D_{wz} + D_{wr} = D_{zr}
\end{equation}
Hence
\begin{align}
    2D_{wy}2^{-g_y} + 2D_{wz}2^{-g_z} + 2D_{wr}2^{-g_w} &= 2D_{wy}2^{-g_y} + 2D_{wz}2^{-g_{z}} + 2D_{wr}(2^{-g_y} + 2^{-g_z})\\
    &= 2(D_{wy} + D_{wr})2^{-g_y} + 2(D_{wz} + D_{wr})2^{-g_z}\\
    &=2D_{yr}2^{-g_y} + 2D_{zr}2^{-g_z}
\end{align}
Thus,
\begin{equation}
    \sum_{X_b(A,B) = 1}D_{AB}2^{-e_{AB}} =\sum_A2^{-g_A}D_{Ar}
\end{equation}
and hence the claim holds by induction as required.
\subsubsection*{Rooting in ultrametric trees}
Under the assumption that distances are additive (that is, one can find the distance between node $A$ and $B$ by summing the lengths of the edges on the path from $A$ to $B$) we make the further assumption that (after scaling) the length of each edge is approximately equal to the amount of time associated with the evolution that occurred on this edge. We use the additional, biologically-motivated assumption that the leaf taxa are being observed at the same point in time. This means that the length in time from the root to each leaf in the tree is the same.

We can then estimate the true length of time from the root to the leaves (i.e. the length of the evolutionary process represented by the tree) from the following simple heuristic. Given two leaf nodes that share a parent, define $d_1$ and $d_2$ to be the length of the edge between each child and its parent. We then approximate the true time between the children's divergence and the current time as $\frac{d_1 + d_2}{2}$. Moreover, if their parent was a distance $d_3$ from its parent, we remove these children from the tree and redefine the edge length between their parent and its parent as $d_3 + \frac{d_1 + d_2}{2}$. 

We can continue this process inductively by continually choosing a pair of sibling leaf nodes, removing them, and updating the distance between their parent and its parent. We stop the process once we have only two leaf nodes remaining, and, if they are distances $d_{n-2}$ and $d_{n-1}$ from the root, we approximate the overall length of the tree to be $\mathcal{D} = \frac{d_{n-2} + d_{n-1}}{2}$.

\textbf{Claim:}
\begin{equation}
    \mathcal{D} = \sum_A2^{-g_A}D_{Ar}
\end{equation}
\textbf{Proof:} This can be proved through induction on the number of nodes. It clearly holds if there are only two nodes in the tree. Assume it holds whenever there are $k$ nodes, and consider a tree with $k+1$ nodes. We process the first pair of leaf nodes, $y$ and $z$, and assume that their associated distances to their parent, $w$ are $D_{wy}$ and $D_{wz}$ and that the new tree created is $\mathcal{T}'$ with distances $D'$. Then, we have, by our inductive hypothesis
\begin{align}
   \mathcal{D} &=   \sum_{A' \in \mathcal{T}'}2^{-g'_{A'}}D'_{A'r'}\\
   &= \sum_{A' \in \mathcal{T}'/\{w\}}2^{-g'_{A'}}D'_{A'r'} + 2^{-g'_w}D'_{wr'}\\
   &= \sum_{A \in \mathcal{T}/\{y,z\}}2^{-g_A}D_{Ar} + 2^{-g_w}\bigg(D_{wr} + \frac{D_{wy} + D_{wz}}{2}\bigg)\\
    &= \sum_{A \in \mathcal{T}/\{y,z\}}2^{-g_A}D_{Ar} + 2^{-g_w}\bigg(\frac{D_{yr} + D_{zr}}{2}\bigg)\\
     &= \sum_{A \in \mathcal{T}}2^{-g_A}D_{Ar}
\end{align}
as required, where we have used the fact that $D_{wr} + D_{wy} = D_{yr}$ and that $2^{g_w} = 2\times2^{-g_y} =2\times2^{-g_z}$.
\subsubsection*{Interpreting the rooting problem}
The previous work has shown that, given an ultrametric \textit{unrooted} tree, the optimal rooting maximises a heuristic for the root-to-tip distance in the tree. Equivalently, the optimal rooting ensures that the root is estimated to be the maximal possible distance back in time.

This is not an immediately biologically plausible objective for the root. Indeed, the cornerstone of BME is that we want the tree of \textit{minimum} length, and it hence seems counter-intuitive to require the root that is the \textit{maximum} distance backwards in time (though, of course, the previous work has showed that this will create the minimum length tree).

However, our assumption of a distant ancestor means that the root of our tree must be the point that is furthest backwards in time. In particular, this means that the evolutionary direction needs to be away from the root. By setting our root such that the root-to-tip distance is maximised, we ensure that the root satisfies this constraint.

This property will not hold if the tree is not ultrametric. If taxa evolve at different rates at different times throughout the tree, then the root will be drawn towards taxa with high evolutionary rates. Thus, caution must be used when applying our rooted algorithm to such trees, although the unrooted algorithm will still give a correct unrooted tree. In this case, it may be best to find the optimal unrooted tree topology and then solve the rooting problem for this tree, rather than finding the optimal rooted tree, as this will reduce the skewing effect of the heterogeneity in evolutionary rates. 
\subsection{Ordered Trees}\label{sec:ordered}
\subsubsection*{Definition}
A tree, $\boldsymbol{v}$, is \textit{ordered} if
\begin{equation}
    v_0 = 0 \quad \text{and} \quad v_i < i \quad \forall i
\end{equation}
As discussed in~\parencite{penn2023}, ordered trees have a number of desirable properties, and are useful for creating efficient phylogenetic optimisation algorithms.
\subsubsection*{A left-to-right construction algorithm for ordered trees}
Under the assumption that $\boldsymbol{v}$ is ordered, it is possible to construct the tree in $\mathcal{O}(n)$ time by processing the nodes from left-to-right (that is, from the lowest-labelled node to the highest-labelled node). This is in contrast to the normal Phylo2Vec algorithm which runs from right-to-left. An example is shown in Fig.~\ref{fig:ltr}.

One can do this by labelling the edges joining each leaf node to the rest of the tree with the same label as the leaf node (that is edge $i$ joins leaf $i$ to the rest of the tree). Then, after initialising with nodes 0 and 1 joined to the root, if $v_j = k$, node $j$ is added to the tree by adding a new internal node on edge $k$ and joining the node $j$ to this edge (so that this new internal node has children $j$ and $k$).

\subsubsection*{Equivalence with Phylo2Vec}
To show that the left-to-right algorithm gives an equivalent tree, define $\mathcal{T}$ to be the tree resulting from the standard Phylo2Vec algorithm and $\mathcal{T}'$ to be the tree resulting from this new left-to-right algorithm. We proceed by induction on the number of nodes, $n$, noting that the case $n=2$ is trivial.
\\
\\
\noindent
Suppose now that the algorithms are equivalent for $n = m$. Choose some ordered $\boldsymbol{v}$ of length $m+1$ (so that this corresponds to $n = m+1$) and consider processing the first node using the Phylo2Vec algorithm, so that (using the fact that $\boldsymbol{v}$ is ordered so that no nodes are skipped), node $m$ merges with node $v_m$. 
\\
\\
\noindent
From this step, the Phylo2Vec algorithm proceeds as if there were $n-1$ nodes and the vector was $\tilde{\boldsymbol{v}} = (v_0,v_1,...,v_{m-1})$. Define $\tilde{\mathcal{T}}$ to be the tree given by $\tilde{\boldsymbol{v}}$. Hence, $\tilde{\mathcal{T}}$ can be created from $\mathcal{T}$ by removing nodes $v_{m}$ and $m$ (and the edges connecting them to the tree) and relabelling their parent as $v_m$. Equivalently (by reversing this process), $\mathcal{T}$ can be created from $\tilde{\mathcal{T}}$ by adding a node to the edge joining leaf node $v_m$ to the tree, and connecting node $m$ to this edge.
\\
\\
\noindent
Moreover, from the inductive hypothesis, $\tilde{\mathcal{T}}$ can be constructed by using the left-to-right algorithm on $\tilde{\boldsymbol{v}}$. As this algorithm processes $v_m$ last, this means that after $m$ nodes have been added to the tree by the left-to-right algorithm applied to $\boldsymbol{v}$, the current tree is given by $\tilde{\mathcal{T}}$. 
\\
\\
\noindent
The final step of the left-to-right algorithm applied to $\boldsymbol{v}$ is to add a node to the edge joining leaf node $v_m$ to the tree, and to connect node $m$ to this edge. As previously discussed, this creates the tree $\mathcal{T}$ and hence, $\mathcal{T} = \mathcal{T}'$ as required.

\subsection{A continuous objective function}
\subsubsection*{Setup}
There exists a natural continuous relaxation of the Phylo2Vec representation. Suppose that the Phylo2Vec vector of a tree is now a random variable $\boldsymbol{V}$. Consider a matrix $W$ where
\begin{equation}
    W_{ij} = \mathbb{P}(V_{i} = j)
\end{equation}
so that $W$ defines the distribution of $\boldsymbol{V}$. We ignore $V_0$ in this construction as it is always equal to $0$. For $i > 0$, $V_i < i$ and so $W$ is a strictly lower-triangular matrix. To denote the dependence of $\boldsymbol{V}$ on $W$, we shall write $\boldsymbol{V} = \boldsymbol{V}(W)$.
\\
\\
\noindent
Given this distribution, one can then calculate the objective function as the expectation of the objective value of a tree drawn with distribution $W$. If $f(\boldsymbol{v})$ is the objective function for a deterministic tree, then one can define
\begin{equation}
    F(W) := \mathbb{E}[f(\boldsymbol{V}(W))]
\end{equation}
If all the lower-triangular entries of $W$ are non-zero, then $\boldsymbol{V}$ can be any ordered tree with non-zero probability. Thus, a naive calculation of this expectation would need to consider the objective values of all $(n-1)!$ ordered trees – a task that quickly becomes computationally infeasible for increasing $n$. However, we can exploit the Phylo2Vec construction to calculate this expectation in $\mathcal{O}(n^3)$, making this method feasible for trees with thousands of taxa.
\subsubsection*{Finding edge lengths (rooted trees)}
The objective function corresponding to the BME model relies on the quantities $2^{-e_{ij}}$, where $e_{ij}$ is the path length between nodes $i$ and $j$ in the tree.
\\
\\
\noindent
We can calculate an exact expectation, $E_{ij} := \mathbb{E}(2^{-e_{ij}})$ for ordered trees by iteratively updating the $E_{ij}$ throughout the left-to-right construction procedure. Adding node $k$ to the tree increases the path length between nodes $i$ and $j$ by 1 if and only if $V_k = i$ or $V_k = j$. As this condition is independent of other values of $\boldsymbol{V}$, using $e_{ij}^k$ to be the path length after the $k$ nodes  $\{0,...,k-1\}$ have been added, one can write
\begin{equation}
    2^{-e^{k+1}_{ij}} =  2^{-(e^{k}_{ij} + \mathds{I}\{V_k \in \{i,j\}\})} =     2^{-e^{k}_{ij}}\times 2^{-\mathds{I}\{V_k \in \{i,j\}\}}
\end{equation}
This is a product of independent random variables and so, defining $E^k_{ij} := \mathbb{E}(2^{-e^k_{ij}})$ and noting that $\mathds{I}\{V_k \in \{i,j\}\}$ is a Bernoulli random variable with probability $W_{ki} + W_{kj}$, this equation becomes
\begin{equation}
\label{eq:iter}
    E^{k+1}_{ij} = E^{k}_{ij} \bigg[(1 - (W_{ki} + W_{kj}) + \frac{1}{2}(W_{ki} + W_{kj})\bigg] =  E^{k}_{ij} \bigg[1 - \frac{1}{2}(W_{ki} + W_{kj})\bigg]
\end{equation}
To close this iterative system, note that when node $j$ is added to the tree, it will be a path length 2 from the leaf node $V_j$ connecting the edge it is joined to. Moreover, the distance between node $j$ and any other nodes $x\neq V_j$ in the tree will be equal to one plus the distance between node $x$ and node $V_j$. That is,
\begin{equation}
    2^{-e_{ij}^{j+1}} = \left\{\begin{matrix} 2^{-(1+e_{i,V_j}^j)} & \text{if $V_j \neq i$} \\
    \frac{1}{4} & \text{if $V_j = i$} \end{matrix} \right.
\end{equation}
Thus, conditioning on the value of $V_j$,
\begin{equation}
\label{eq:init}
    E_{ij}^{j+1} = \bigg[\frac{1}{2}\sum_{x\neq i}E_{ix}^jW_{jx}\bigg] + \frac{1}{4}W_{ji}
\end{equation}
Finally, by symmetry, $E_{ji}^{j+1} = E_{ij}^{j+1}$. Noting that $E_{ij}^k$ is undefined (and unnecessary) for $k < \max(i,j) + 1$, as nodes $i$ and $j$ have not both been added to the tree, (\ref{eq:iter}) and (\ref{eq:init}) hence form a closed system. This can be solved inductively, finding all $E_{ij}^m$ terms for $m=2,3,...,n$.
\\
\\
\noindent
To find the $E^m_{ij}$ terms, there are $\mathcal{O}(m)$ steps of $\mathcal{O}(m)$ (finding the $E_{m-1, j}^m$ terms) and $\mathcal{O}(m^2)$ steps of $\mathcal{O}(1)$ (finding the other $E_{ij}^m$ terms). There are $\mathcal{O}(n)$ values of $m$ that need to be considered, and hence this system can be solved in $\mathcal{O}(n^3)$ time.
\\
\\
\noindent
Note that this method would not work in the case of unordered trees (in effect, this would be make it possible that new nodes are added to edges not connected to leaves). If node $k$ were joined to some internal edge $x$, then $e_{ij}$ would increase if edge $x$ were on the path from $i$ to $j$. However, this is clearly not independent of $e_{ij}^k$, and hence a similar iterative scheme cannot be derived.
\subsubsection*{Objective function}
The objective function for BME is then
\begin{equation}
\label{eq:continuous_in_D}
    F(W) := \mathbb{E}\bigg[\sum_{i\neq j}2^{-e^{n}_{ij}}D_{ij}\bigg] = \sum_{i\neq j}D_{ij}E_{ij}
\end{equation}
And the overall computation time remains $\mathcal{O}(n^3)$ time (which is dominated by the calculation of the $E_{ij}$ terms).
\subsubsection*{Unrooted trees}
It may be preferable to calculate this objective for an unrooted tree. This can be done from the same construction, but where initially, nodes 0 and 1 are a distance 1 away from each other (rather than distance 2 in the rooted case). This, in effect, gives the edges that join the root a weight of $\frac{1}{2}$ rather than $1$, hence producing the correct path lengths. Thus, the only difference to the edges algorithm is that $E^2_{01} = \frac{1}{2}$ rather than $\frac{1}{2}$, and the rest of the algorithm proceeds identically (as, for example, adding a node to edge 0 still increases the distance between node 0 and all other nodes by 1).
\subsection{Properties of the continuous objective function}\label{sec:continuous_objective}
\subsubsection*{Recovering the discrete objective function}
To recover the objective value of a deterministic tree $\boldsymbol{v}$, one can set
\begin{equation}
    W_{ij} = \mathds{I}\{v_i = j\}
\end{equation}
This means that $\boldsymbol{V}(W) = \boldsymbol{v}$ and hence $f(\boldsymbol{v}) = F(W)$
\subsubsection*{Discreteness of optima}
Noting that $F(W)$ comes from an expectation, one can rewrite it as
\begin{align}
\label{eq:Fbig}
    F(W) &= \sum_{\boldsymbol{v}}\mathbb{P}(\boldsymbol{V} = \boldsymbol{v})f(\boldsymbol{v})\\
    \label{eq:vsplit} &=  \sum_{\boldsymbol{v}}\bigg(\prod_{i=0}^{n}W_{i, v_i}\bigg)f(\boldsymbol{v})
\end{align}
Noting that
\begin{equation}
\sum_{\boldsymbol{v}}\bigg(\prod_{i=1}^{n}W_{i-1, v_i}\bigg) = \sum_{\boldsymbol{v}}\mathbb{P}(\boldsymbol{V} = \boldsymbol{v}) = 1
\end{equation}
this means that the objective function is a weighted average of the objective values of all the deterministic trees. Thus, in particular, it is minimised when
\begin{equation}
    \mathbb{P}\bigg(\boldsymbol{V} \in \{\boldsymbol{v} : f(\boldsymbol{v}) = \min_{\boldsymbol{s}}(f(\boldsymbol{s})\}\bigg) = 1
\end{equation}
In general, the minimum of $f$ is achieved at a unique tree, $\boldsymbol{v}^*$ and hence, $F(W)$ is minimised when
\begin{equation}
    \mathbb{P}(\boldsymbol{V} = \boldsymbol{v}^*) = 1
\end{equation}
That is, it is minimised when $\boldsymbol{V}$ is deterministically equal to the optimal tree. Thus, minimising $F$ gives the same tree as minimising $f$.
\subsubsection*{Finding $\nabla F$}
Note that, from (\ref{eq:Fbig}), $F$ is linear in each variable $W_{ij}$ (when other variables are fixed). Thus, for any $\epsilon > 0$,
\begin{equation}
  (\nabla F)_{ab} =\frac{F(W + \epsilon X(a,b)) - F(W)}{\epsilon}
\end{equation}
where $X(a,b)$ is a matrix with $(a,b)$ entry equal to 1 and all other entries equal to 0. This is exact for all $\epsilon$ rather than approximate for small $\epsilon$ because of the linearity. Similar calculations can be made for the Hessian (and indeed higher derivatives). Note that the matrix $W + \epsilon X(a,b)$ lacks phylogenetic interpretability, but nevertheless can be assigned a value of $F$ for finding the gradient.
\subsubsection*{Single-step approximation}
One can approximate the optimal ordered tree after a single gradient step from a uniformly distributed tree.
\\
\\
\noindent
To show this, consider the objective function as written in (\ref{eq:vsplit}). That is,
\begin{equation}
F(W) =  \sum_{\boldsymbol{v}}\bigg(\prod_{i=0}^{n}W_{i, v_i}\bigg)f(\boldsymbol{v})
\end{equation}
Note that
\begin{equation}
    (\nabla F)_{ab} = \sum_{\boldsymbol{v} : v_a = b}\bigg(\prod_{i\neq a}W_{i, v_i}\bigg)f(\boldsymbol{v})
\end{equation}
As the distribution is uniform, the product $\prod_{i\neq a}W_{i, v_i}$ is independent of $\boldsymbol{v}$ and hence
\begin{equation}
 (\nabla F)_{ab} =  \sum_{\boldsymbol{v} : v_a = b}f(\boldsymbol{v})
\end{equation}
In a single-step optimisation procedure, the value of $v_a$ is set to
\begin{equation}
    v_a = \text{argmin}_b\bigg\{(\nabla F)_{ab} \bigg\} = \text{argmin}_b\bigg\{ \sum_{\boldsymbol{v} : v_a = b}f(\boldsymbol{v}) \bigg\}
\end{equation}
In general, this is a sensible heuristic – setting one of the elements in a uniformly-chosen tree to be equal to its optimal value will often decrease the objective. Fig.~\ref{fig:big_jump} shows how it can successfully recover the optimal tree from an even a random starting point (given a correct ordering – discussed below), which requires a large number of changes to the tree topology. However, one must use more sophisticated gradient-based algorithms to reliably find the optimal ordered tree for more complicated phylogenies.
\subsection{Orderings}
The continuous objective function is only defined for ordered trees, which, for a given labelling of the nodes, is a subset of the whole tree space. Thus, we define the concept of an \textit{ordering} of the nodes and changing the ordering will allow the full space of trees to be explored.

\subsubsection*{Definition}
Suppose that the nodes correspond to taxa with names $N_0,N_1,...N_{n-1}$. We then define an \textit{ordering} of the nodes to be a permutation, $\sigma$ of the set $\{0,...,n-1\}$ such that the node with name $N_i$ is processed as node $\sigma(i)$ by the Phylo2Vec algorithm. It is necessary that the associated Phylo2Vec vector $\boldsymbol{v}(\sigma)$ is ordered.

Note that we use the phrase “node $x$'' to mean “the node with name $N_x$'' and will always be explicit if we refer to a node by its label.

\subsubsection*{Generating an ordering from a tree}
Given a tree, it is possible to generate a possible ordering of the nodes, $\sigma$, as well as the associated vector $\boldsymbol{v}(\sigma)$. We will do this by labelling the tree, again distinguishing between the leaf node names $N_i$ and their labels, which we will call $l(i)$. 
\\
\\
\noindent
Consider labelling the root node as 0. Then, label the children of this node as $0$ and $1$. One can continue this process inductively, choosing a node, labelled $x$, with unlabelled children and then labelling its children as $x$ and $y$, where $y$ is the smallest unused label. Continue this process until every node has been labelled, and, as discussed above, suppose that the label of the leaf node with name $N_i$ is $l(i)$.
\\
\\
\noindent
\textsb{Claim 1:} Two nodes have the same label only if they share an ancestor with that label.
\\
\\
\noindent
\textsb{Proof:} Suppose that this is false, and that nodes $x$ and $y$ have the same label, $L$, but do not share an ancestor with that label. Define $a(x)$ and $a(y)$ to be the nodes of lowest generation (that is, the nodes closest to the root) with label $L$ such that they are ancestors of $x$ and $y$ respectively. Note that, by assumption, $a(x) \neq a(y)$ and also, neither can be the root (as the root is the ancestor of all nodes). Moreover, they cannot share a parent, as the children of a parent are labelled differently. Thus, without loss of generality, one can assume that $a(x)$ was labelled first. By definition, the parent of $a(x)$ does not have label $L$ and hence, $L$ must have been the smallest unused label when node $a(x)$ was labelled. A similar argument for $a(y)$ shows that $L$ must have been the smallest unused label when node $p(y)$ was labelled. However, when node $a(y)$ was labelled, $L$ had been used to label $a(x)$, giving the required contradiction.
\\
\\
\noindent
\textsb{Claim 2:} $l$ is a permutation of the set $\{0,1,...,n-1\}$.
\\
\\
\noindent
\textsb{Proof:} Firstly, note that as there are $n-1$ internal nodes, and a single new label is introduced every time the children of an internal node are labelled, the set of labels used (across all nodes) must be $\{0,1,...,n-1\}$.
\\
\\
\noindent
Suppose that leaf nodes $x$ and $y$ have the same label $L$. By the previous claim, they must share an ancestor $a$ with that label. Define $b$ to be the shared ancestor with the highest generation (that is, furthest from the root) such that $b$ has label $L$. Then, either nodes $x$ and $y$ are the children of $b$ (in which case, they have distinct labels) or they are descendants of distinct children, $c$ and $d$, of $b$. In the second case, one can impose without loss of generality that $c$ does not have label $L$ and, as label $L$ has already been used to label $b$, we know that all descendants of $c$ do not have label $L$. Hence, in both cases, one of $x$ and $y$ does not have label $L$ as required.
\\
\\
\noindent
\textsb{Claim 3:} For each $i \in \{0,1,...,n-1\}$, define $x(i)$ to be the node of the highest generation with label $i$. Define (for $i > 0$), $y(i)$ to be the label of the parent of $x(i)$. Then, with ordering $l$, the tree is given by
\begin{equation}
    v_0 = 0 \quad \text{and} \quad v_{i} = y(i) \quad \forall i > 0
\end{equation}
\textsb{Proof:} Firstly, note that $\boldsymbol{v}$ is ordered, as the label of a child is greater than or equal to that of its parent. Hence, as the parent of $x(i)$ does not have label $i$, it must have a label strictly less than $i$ and so $v_i < i$ as required.
\\
\\
\noindent
Consider constructing the tree according the “standard'' right-to-left Phylo2Vec algorithm. One can then proceed by induction on the number of nodes. The case $n=2$ is trivial, and so suppose it holds for $n = m$ and consider a tree with $n = m+1$.
\\
\\
\noindent
The first node, $x$, to be processed has label $m$. The parent of the node with label $m$ cannot also have label $m$ (as, otherwise, its other child would have label greater than $m$, contradicting Claim 2). Similarly, no other node in the tree can have label $m$ and hence, the parent of $x$ must have label $y(m)$.  This must also be the label of its other child and hence, $v_m = y(m)$ ensures that the node with label $m$ merges with its sibling from the original tree (which is correct). 
\\
\\
\noindent
From this point, the tree now has $m$ nodes, and our right-to-left construction algorithm considers the parent of the node labelled $m$ to now be a leaf node with label $y(m)$. The values of $y(i)$ for this tree are unchanged (in particular, $y(y(m))$ depends on the label of an ancestor of the parent of node $m$) and hence, by induction, the remaining values of $\boldsymbol{v}$ correctly generate the rest of the tree. Thus, the correct tree is generated by $\boldsymbol{v}$ as required.
\subsubsection*{The number of possible orderings for a tree}
Given a tree, one can use the previous labelling algorithm to show that there are at least $2^{n-1}$ possible orderings for the tree (as the children of each node can be labelled in either order). The exact number depends on the choice of which internal node is processed at each step (and so, a “flat'' tree where the leaves have a low generation has more possible orderings than a “ladder'' tree where each leaf has a distinct generation). However, in general, it will be substantially larger than $2^{n-1}$ (we conjecture that for flat trees, it may be factorial in size) and hence there are numerous possibilities which will allow for a global minimum of the objective to be found.
\subsection{Queue Shuffle: generating principled ordering proposals}\label{sec:queue_shuffle}
\subsubsection*{The importance of well-chosen orderings}
While the number of possible orderings for the optimal tree is large, the proportion of these orderings falls quickly as $n$ increases. An estimate for this proportion is
\begin{equation}
    \text{Proportion of optimal orderings} \approx \frac{\text{Trees per ordering}}{\text{Total trees}} = \frac{(n-1)!}{(2n-3)!!}
\end{equation}
which is exponentially decreasing in $n$. The exact value will depend on the “flatness'' of the optimal tree. Thus, it is crucial to efficiently explore the space of possible orderings to find the optimal tree, as the number of uniformly chosen orderings needed to find the optimal tree will quickly become computationally impractical.

 One way to increase efficiency is to ensure that the previous best tree is in the new space of ordered trees. That is, suppose that $\mathcal{T}$ is the optimal ordered tree for the current ordering. The algorithm in the previous section provides a method for choosing a new random ordering, by randomising the order in which nodes are processed and randomising which of the children is given the same label as their parent. $\mathcal{T}$ will still be in the space of ordered trees, and hence re-optimising in this new ordered space will not increase the objective value (provided the true optimal ordered tree is found).

However, even choosing the new ordering from a uniform distribution over the space of orderings containing $\mathcal{T}$ will lead to inefficient optimisation as $n$ grows. In the optimisation scheme used in this paper, we use the topology of $\mathcal{T}$ to further inform the distribution of the next ordering that is proposed. The true optimal tree is likely to be reasonably “close'' to $\mathcal{T}$ (especially after a few initial iterations of the algorithm) and so it is important to choose a new ordering such that allows for a thorough exploration of the space of these “close'' trees.
\subsubsection*{Asymmetry of ordered tree spaces}
A key feature of the Phylo2Vec construction that can be exploited to make sensible ordering proposals is the “asymmetry'' of ordered tree space. That is, in a uniformly chosen tree from an ordered tree space, nodes with low labels are likely to be closer to the root.

This can be shown as follows. Define $g_k^m$ to be the expected distance from the root of the node labelled $m$ in a tree with $k$ nodes. Then, from our left-to-right construction algorithm,
\begin{equation}
\label{eq:init_eq}
    g^k_{k-1} = \sum_{m=0}^{k-2}\frac{1}{k-1} (1+g^{k-1}_m)
\end{equation}
as adding node $v_{k-1} = m$ means that the path length between node $k-1$ and the root will be one more than the path length of between $m$ and the root. If $v_{k-1} = m$, it will also increase the path length between node $m$ and the root by 1 and so
\begin{equation}
    g^k_m = \frac{k-2}{k-1}g^{k-1}_m + \frac{1}{k-1}(g^{k-1}_m + 1) = g^{k-1}_m + \frac{1}{k-1}
\end{equation}
The initial conditions of this system are that
\begin{equation}
    g_0^2 = g_1^2 = 1
\end{equation}
as in a two-node rooted tree, the leaves are distance 1 from the root. Given the harmonic sum function
\begin{equation}
    H(m) = \left\{ \begin{matrix} \sum_{j=1}^m\frac{1}{j} &\text{if $m \geq 1$}\\ 1 & \text{if $m=0$}\end{matrix}\right.
\end{equation}
we claim that the solution to this system is
\begin{equation}
    g^k_m =H(k-1) + H(m) - 1
\end{equation}
where $H(0) = 0$. Note that this holds for $k = 2$ as $H(1) = H(0) = 1$. Moreover, under the inductive hypothesis that it holds for $k-1$,
\begin{equation}
     g^k_m = g^{k-1}_m + \frac{1}{k-1} =  H(k-2) + H(m) - 1 + \frac{1}{k-1} = H(k-1) + H(m) - 1
\end{equation}
and
\begin{align}
    g^k_{k-1} &= \sum_{m=0}^{k-2}\frac{1}{k-1} (1+g^{k-1}_m)\\
    &= \sum_{m=0}^{k-2}\frac{1}{k-1} (1 + H(k-2) +H(m) - 1)\\
    &= \sum_{m=0}^{k-2}\frac{1}{k-1}(H(k-2) + H(m))\\
    &= H(k-2) + \frac{1}{k-1}\sum_{m=0}^{k-2}H(m)\\
    &= H(k-1) + \frac{1}{k-1}\sum_{m=1}^{k-2}\sum_{j=1}^m\frac{1}{j}
\end{align}
Now,
\begin{equation}
    \sum_{m=1}^{k-2}\sum_{j=1}^m\frac{1}{m} = \sum_{j=1}^{k-2}\sum_{m = j}^{k-2}\frac{1}{j} = \sum_{j=1}^{k-2}\frac{k-1-j}{j} = (k-1)H(k-2) -(k-2)
\end{equation}
and hence
\begin{equation}
     g^k_{k-1} = H(k-1) + H(k-2) -\frac{(k-2)}{(k-1)} = H(k-1) + H(k-1) - 1
\end{equation}
as required.

Thus, the expected distance from the root grows harmonically as the label increases. For large trees, the node with label $n-1$ has an expected distance from the root of approximately twice the expected distance from the root of the node label $0$. This property is noticeable even for small trees – if $n = 10$, then $g^{10}_9/g^{10}_0 = 1.65$.
\subsubsection*{Queue Shuffle}
Our ordering proposal algorithm, \textit{Queue Shuffle}, exploits this asymmetry to improve the efficiency with which we explore different orderings. In BME, the dominant contribution to the objective function generally comes from the nodes which are closest to the root (as these will have larger $D_{ij}$ values than the order nodes). Thus, it is reasonable to expect that the true outgroups will be close to the root in the optimal tree in any ordering and, therefore, nodes close to the root should be given low labels in our new ordering.

Queue Shuffle uses a version of the previously discussed ordering algorithm such that the set of internal nodes with a given generation (that is, a given distance from the root) are processed consecutively. That is, we begin by processing all nodes with generation 0 (i.e., the root), then all internal nodes with generation 1, then all internal nodes with generation 2, and continue in this fashion until all internal nodes have been processed.
\\
\\
\noindent
Algorithmically, this can be achieved by a “queue'' of internal nodes to be processed. When an internal node is processed, any of its children that are also internal nodes are added to the back of this queue. Thus, the queue is always in ascending order of generation, and it is simple to show that this ensures the required property. 
\\
\\
\noindent
A crucial feature of this queue is that the child given the same label as its parent is placed \textit{ahead} of the other child in the queue. This ensures that one can, in some way, control the order of processing by choosing the labelling of the children of each node. Moreover, it is vital for the theoretical result presented in the following section. 
\\
\\
\noindent
To add randomness into the labelling procedure, every time an internal node is processed, we randomly choose which child is given the label of their parent, and which child is given the next available label. This provides $2^{n-1}$ possible orderings for each tree. This stochasticity is helpful in ensuring that the algorithm does not get stuck – as discussed in the subsequent section, it ensures that a large class of similar trees will be considered after a small number of ordering proposals.
\subsubsection*{The Swapping Property}
Queue Shuffle is an extremely powerful algorithm, as it allows for great flexibility in exploring tree space, while also keeping a sense of continuity between the sets of ordered trees under consideration. This is exemplified by the \textit{Swapping Property}, which is the fact that subtrees attached to internal nodes sharing an edge can be swapped with probability at least $\frac{1}{4}$, irrespective of the total number of nodes in the tree.

This property is illustrated in Fig.~\ref{fig:swap} and formalised in Theorem 1. To do this, it is necessary to have the following definitions

\textbf{Definition:} Define $\tau(\sigma)$ to be the space of possible trees given an ordering $\sigma$. 
\\
\\
\noindent
\textbf{Definition:} For a tree $\mathcal{T}$, define $Q(\mathcal{T})$ to be the random ordering generated by Queue Shuffle. 
\\
\\
\noindent
\textbf{Definition:} Finally, define two internal nodes to be \textit{joined} if they share an edge.
\\
\\
\noindent
\textbf{Theorem 1:} \textit{Consider a tree $\mathcal{T}$. Choose two joined internal nodes, $i$ and $j$ and suppose without loss of generality that $i$ is the parent of $j$. Suppose that the other child of $i$ is the root of a subtree $\mathcal{S}_i$, and that a child of $j$ is the root of the subtree $\mathcal{S}_{j}$. Finally, generate $\mathcal{T}'$ from $\mathcal{T}$ by swapping $\mathcal{S}_i$ and $\mathcal{S}_j$. Then,}
\begin{equation}
    \mathbb{P}\bigg[\mathcal{T}'\in \tau\bigg(Q(\mathcal{T})\bigg)\bigg] \geq \frac{1}{4}
\end{equation}
To facilitate the proof, it is first helpful to prove two lemmas.
\\
\\
\noindent
\textbf{Lemma 1.1:} \textit{For a given permutation $\sigma$},
\begin{equation}
\label{eq:equallike}
    \mathbb{P}\bigg[Q(\mathcal{T}) = \sigma\bigg] \in \bigg\{0,\frac{1}{2^{n-1}}\bigg\}
\end{equation}
\textbf{Proof 1.1} Suppose that every (internal and external) node in $\mathcal{T}$ is assigned a fixed unique position, such that one can consistently define a “leftmost'' and “rightmost'' node from a pair of nodes. Then, the randomness in the Queue Shuffle algorithm can be represented by a uniform random vector $\boldsymbol{r} \in \{0,1\}^{n-1}$ such that when the $m^{\text{th}}$ internal node is processed, the leftmost child is given the same label as its parent if and only if $r_{m+1} = 1$. Each distinct $\boldsymbol{r}$ results in a distinct ordering (as, given the leaf labels, one can generate the unique labelling of the tree as a parent must have a label equal to the minimum of the labels of its two children). Hence, each possible labelling is equally likely, giving (\ref{eq:equallike}) and completing the proof.

For a given permutation $\sigma$, define $l_i({\sigma})$ to be the label assigned to node $i$, $l_j({\sigma})$ to be the label assigned to node $j$,  $l^{\mathcal{S}}_i({\sigma})$ to be the label assigned to the root of $\mathcal{S}_i$ and $l^{\mathcal{S}}_j({\sigma})$ to be the label assigned to the root of $\mathcal{S}_j$. Suppose that the other child of node $j$ is node $c$, and suppose it has label $l_c(\sigma)$
\\
\\
\noindent
This allows a further lemma to be proved about the labels of node $i$, $j$ and their children. 
\\
\\
\noindent
\textbf{Lemma 1.2:} 
\begin{equation}
    \mathbb{P}\bigg[l^{\mathcal{S}}_j({Q(\mathcal{T})})  =l_i({Q(\mathcal{T})})  \bigg] = \frac{1}{4}
\end{equation}
\textbf{Proof 1.2:} Using the $\boldsymbol{r}$ defined in the proof of Lemma 1.1, define the random indices $A$ and $B$ such that $r_A$ corresponds to processing node $i$ and $r_B$ corresponds to processing node $j$. Note that $r_A$ and $r_B$ are independent (though $B$ will in general depend on $r_A$). 
\\
\\
\noindent
Now, suppose without loss of generality that $j$ is the leftmost child of $i$ and that the root of $\mathcal{S}_j$ is the leftmost child of $j$. As children have labels greater than or equal to their parents, 
\begin{equation}
     \mathbb{P}\bigg[l^{\mathcal{S}}_j({Q(\mathcal{T})})  =l_i({Q(\mathcal{T})})\bigg] = \mathbb{P}\bigg[l^{\mathcal{S}}_j({Q(\mathcal{T})})  = l_j({Q(\mathcal{T})})  =l_i({Q(\mathcal{T})})\bigg]
\end{equation}
and hence
\begin{equation}
     \mathbb{P}\bigg[l^{\mathcal{S}}_j({Q(\mathcal{T})})  =l_i({Q(\mathcal{T})})\bigg] = \mathbb{P}(r_A = r_B = 1) = \frac{1}{4}
\end{equation}
which is the required result.
\\
\\
\noindent
\textbf{Proof of Theorem 1:} Suppose for a permutation $\sigma$ that $l^{\mathcal{S}}_j(\sigma)  =l_i(\sigma)$. Necessarily (as $r_B = 0$), $l_c(\sigma)$ was the smallest available label when processing node $j$, which must be bigger than the smallest available label when node $i$ was processed (as $j$ is the child of $i$ and hence processed later). Thus, $l_c(\sigma) >l^{\mathcal{S}}_i(\sigma)$. 
\\
\\
\noindent
A further important property is that, as $r_A = 1$ (to ensure $l^{\mathcal{S}}_j(\sigma)  =l_i(\sigma)$), node $j$ must have been placed ahead of the root of $\mathcal{S}_i$ in the queue. Thus, all nodes in $\mathcal{S}_i$ are labelled either as $l^{\mathcal{S}}_i(\sigma)$ or with a label that is greater than $l_c(\sigma)$, as all internal nodes in $\mathcal{S}_i$ are processed after node $j$. Moreover, all nodes in $\mathcal{S}_j$ are labelled as either $l^{\mathcal{S}}_j(\sigma)$ or a label greater than $l_c(\sigma)$ as they were processed after node $j$.
\\
\\
\noindent
Define  $\boldsymbol{v}$ to be the vector giving $\mathcal{T}$ under $\sigma$. Then, define a new vector $\boldsymbol{v}'$ by
\begin{equation}
    v'_{m} =\left\{ \begin{matrix} l^{\mathcal{S}}_i(\sigma) & \text{if $m =l_c(\sigma) $}\\
    v_m & \text{otherwise} \\
    \end{matrix}\right.
\end{equation}
Then, $\boldsymbol{v}'$ is ordered as $l_c(\sigma) > l_j^{\mathcal{S}}(\sigma)$. We now show that $\boldsymbol{v}'$ generates $\mathcal{T}'$ by using the left-to-right construction algorithm. Note that up to the point that node $l_c(\sigma)$ is processed by this algorithm, no nodes have appended to the edges connecting either the root of $\mathcal{S}_i$ or $\mathcal{S}_j$ to the tree. This holds because all other nodes in $\mathcal{S}_i$ and $\mathcal{S}_j$ have labels greater than $l_c(\sigma)$. Changing from $\boldsymbol{v}$ to $\boldsymbol{v}'$ means that the leaf node labelled $l_c(\sigma)$ is joined to the edge connecting the root of $\mathcal{S}_i$ rather than the root of $\mathcal{S}_j$. The rest of the tree is then constructed identically as the vectors $\boldsymbol{v}$ and $\boldsymbol{v}'$ are the same.
\\
\\
\noindent
Thus, changing from $\boldsymbol{v}$ to $\boldsymbol{v}'$ involves removing the subtree rooted at $c$ from the edge connecting $j$ and the root of $\mathcal{S}_j$ and regrafting it to the tree on the edge connecting $i$ and the root of $\mathcal{S}_i$. This is topologically equivalent to switching $\mathcal{S}_i$ and $\mathcal{S}_j$, as shown in Fig.~\ref{fig:swap}.
\\
\\
\noindent
This completes the proof as it shows that
\begin{equation}
     \mathbb{P}\bigg[\mathcal{T}'\in \tau\bigg(Q(\mathcal{T})\bigg)\bigg| l^{\mathcal{S}}_j(\sigma)  =l_i(\sigma)\bigg] =1
\end{equation}
and hence, by Lemma 1.2
\begin{equation}
    \mathbb{P}\bigg[\mathcal{T}'\in \tau\bigg(Q(\mathcal{T})\bigg)\bigg] \geq  \mathbb{P}\bigg[\mathcal{T}'\in \tau\bigg(Q(\mathcal{T})\bigg)\bigg| l^{\mathcal{S}}_j(\sigma)  =l_i(\sigma)\bigg]\mathbb{P}\bigg[l^{\mathcal{S}}_j(\sigma)  =l_i(\sigma)\bigg] = \frac{1}{4}
\end{equation}

\subsection{Eutherian Mammal phylogeny~\parencite{Song2012-ql}}
\FloatBarrier
\input{fig/figS1}

\clearpage
\subsection{Convergence analysis}
Figure~\ref{fig:convergence_analysis} compares the performance of different optimisers (Adafactor~\parencite{shazeer2018}, AdamW~\parencite{loshchilov2018}, RMSprop~\parencite{tieleman2012}, and SGD) under different DNA substitutions models (JC69~\parencite{jukes1969}, F81~\parencite{felsenstein1981}, TN93~\parencite{tamura1993}) on a single optimisation step (no subsequent reordering with Queue Shuffle) for a maximum of 5000 steps. Four learning rates were considered, logarithmically spaced from 0.001 to 1.0. Whereas convergence speed appears to be independent of the chosen DNA substitution model, the results varied widely with respect to the optimisation algorithm. In particular, Adafactor optimisation produced the best performance, with increasing convergence speed as learning rates were higher.

\input{fig/figS2}
